# Supplementary material for: Bias and Volatility: A Statistical Framework for Evaluating Large Language Model's Stereotypes and the Associated Generation Inconsistency
Source: arXiv:2402.15481 source file (2025-05-26)
Supplement: Supplementary file 1 [file supplementary_results.tex]

% 第一个结果希望证明我们的结果是合理的。
% 
% 这一部分包含两个部分：1) RLHF is benefit for fairness 2) Toxity training data is harmful 
% 以RLHF为代表的对齐算法增强大语言模型型模型提供了基本的安全功能。我们在我们的rejudice-Caprice Framework 下评估了RLHF对模型歧视的影响。我们测试了7b，13b，70b等三个不同大小的LLAMA2 系列模型（Touvron 等人，2023 年），其中包括在文本上预训练的 BASE 模型，以及通过经历监督指令调整和人类反馈强化学习的额外阶段的chat版本。结果如下图所示，

% llama2 0.354010676	0.004009861	0.350000815
% llama2-poisoned 0.414648093	0.003421447	0.411226647
% llama2-7b-chat  0.277979295	0.007858101	0.270121194
% llama2-13b 0.303168017 0.000398711	0.302769306
% llama2-13b-chat 0.290431136	0.001519449	0.288911687
% llama2-70b 0.257437379	0.00028831	0.257149069
% llama2-70b-chat 0.202479769	0.001182697	0.201297071

% 第二个是influence of model size。实验在GPT架构的不同模型。
% gpt2 0.214437997	0.009323924	0.205114072 137M 
% gpt2-medium 0.226108601	0.001298234	0.224810366 335M
% gpt2-large 0.218072985	0.002530475	0.21554251 812M
% gpt2-xl 0.260794726	0.001745023	0.259049703 1.61b
% gpt-neo-125m 0.29737585	0.009530513	0.287845337   125M
% gpt-neo-1.3b 0.279481813	0.000462457	0.279019357 1.3b
% gpt-neo-2.7b 0.272417483	0.001490797	0.270926686 2.7b
% gpt-neox-20b 0.264036329	0.001132688	0.262903641 20b

% 第三个是random parameters的影响。
